# Supplementary material for: Mogao: An Omni Foundation Model for Interleaved Multi-Modal Generation
Source: arXiv:2505.05472 source file (2025-05-11)
Supplement: Supplementary file 1 [file appendix.tex]

\section{Hello World}
%\subsection{Hello World}
